# Supplementary material for: Model-Free Optimal Voltage Control via Continuous-Time Zeroth-Order Methods
Source: arXiv:2103.14703 source file (2021-03-26)
Supplement: Supplementary file 1 [file Appendix2.tex]

\appendix

\subsection{The Complete Results and Proof}
The proof of Theorem \ref{thm:spas} follows as a particular case of the next general result for extremum seeking control based on ODEs with a continuous (not necessarily Lipschitz) right-hand side:
\begin{theorem}\label{general_theoremES}
Consider the following closed-loop system:
\begin{subequations}\label{closed_loopESGeneral}
\begin{align}
\dot{z}_1&= kF(z_1,z_2),\\
\dot{z}_2&=\frac{1}{\varepsilon_f}\left(-z_2+\frac{2}{\varepsilon_a}J(z_1+\varepsilon_a\mathbb{D}z_3)\mathbb{D}z_3\right),\\
\dot{z}_3&=\frac{2\pi}{\varepsilon_p} \Pi(\kappa)z_3\label{oscillatordynamics}
\end{align}
\end{subequations}
evolving in the set $\mathcal{Z}\times\mathbb{R}^n\times\mathbb{T}^n$. Suppose the following holds:
\begin{enumerate}
    \item The vector of parameters $\mathbf{\kappa}$ satisfy $\kappa_l\neq\kappa_i$, where each $\kappa_l$ is a positive rational number. 
    \item The function $F$ is continuous, the set $\mathcal{Z}$ is closed, and the dynamical system 
    \begin{equation}\label{nominalAverage}
    \dot{y}_1=F(y_1,\nabla J(y_1)),
    \end{equation}
    renders the set $\mathcal{Z}$ forward invariant. Moreover, there exists a compact set $\mathcal{A}\subset\mathbb{R}^n$ and a function $\beta_1\in\mathcal{K}\mathcal{L}$ such that $\nabla J(\mathcal{A})=0$ and every solution of \eqref{nominalAverage} with $z_1(0)\in\mathcal{Z}$ satisfies
    \begin{equation}\label{KLboundTheorem}
        |z_1(t)|_{\mathcal{A}}\leq \beta_1(|z_1(0)|_{\mathcal{A}},t),
    \end{equation}
    for all $t\geq0$.
\end{enumerate}
Then, for each pair $\Delta>\nu>0$ there exists $\varepsilon_f^*>0$ such that for each $\varepsilon_f\in(0,\varepsilon_f^*)$ there exists $\varepsilon_a^*>0$ such that for each $\varepsilon_a\in(0,\varepsilon_a^*)$ there exists $\varepsilon_p^*$ such that for all $\varepsilon_p\in(0,\varepsilon_p^*)$, every solution of \eqref{closed_loopESGeneral} with initial condition $z(0)\in \left[(\mathcal{A}+\Delta\mathbb{B})\cap\mathcal{Z}\right]\times \Delta\mathbb{B}\times\mathbb{T}^n$ satisfies
\begin{equation}
         |z_1(t)|_{\mathcal{A}}\leq \beta_1(|z_1(0)|_{\mathcal{A}},t)+v,~~\forall~t\geq0,
\end{equation}
and $\limsup_{t\geq0}|z_2(t)|\leq\nu$. \hfill\qedsymbol

\end{theorem}
\noindent 
\textbf{Proof}: The proof uses singular perturbation tools from \cite{} and \cite{}, as well as some auxiliary constructions used to guarantee completeness of solutions for the system. 
\begin{lemma}\label{auxlemmagradient}
For each $\epsilon>0$ there exists $\delta>0$ such that
\begin{equation}
   |z_1^A|_{\mathcal{A}}\leq \delta\implies |\nabla J(z^A_1)|\leq \epsilon.
\end{equation}
\end{lemma}
\noindent
\textbf{Proof:} The results follows by the fact that $\nabla J(\mathcal{A})=0$, and by continuity of $\nabla J$.  \hfill$\blacksquare$ 

\vspace{0.1cm}
The next Lemma, which follows as a particular case of \cite[Lemma 5]{NunoShamma_2020}, will be instrumental for our results. 
\begin{lemma}\label{auxiliarylemma}
Let $\tilde{M}>0$ be given, and let $u:\mathbb{R}_{\geq0}\to \tilde{M}\mathbb{B}$. Then, for any $s>0$ the set $\tilde{M}\mathbb{B}$ is forward invariant under the dynamics $\dot{z}_2=s(-z_2+u(t))$. \hfill\qedsymbol
\end{lemma}
Let $k$, $\Delta$ and $\nu$ be given, where without loss of generality we assume that $\nu\in(0,1)$. Define the set
\begin{equation}\label{KLboundproof}
\mathcal{F}_s:=\left\{z_1\in\mathcal{Z}:|z_1|_{\mathcal{A}}\leq \beta_{1}\left(\max_{y\in \mathcal{A}+\Delta\mathbb{B}}|y|,0\right)+1\right\}.
\end{equation}
Since without loss of generality we can take $\beta_1$ to be continuous, the set $\mathcal{F}_s$ is compact. It follows that $\mathcal{F}_s$ is bounded, in the sense that there exists $M$ such that $\mathcal{F}_s\subset M\mathbb{B}$. Since $J$ is $C^2$, the gradient  $\nabla J$ is continuous, which implies the existence of a positive constant $\tilde{M}>\max\{1,\Delta\}$ such that $|z_1|\leq M$ implies $|\nabla J(z_1)+1|\leq \tilde{M}$. Let $C:=\mathcal{F}_s\times\bar{M}\mathbb{B}$, where $\bar{M}=\tilde{M}+1$. Note that $C$ is compact by construction. Using this set, we first study the behavior of system \eqref{closed_loopESGeneral} restricted to evolve in $C\times\mathbb{T}^n$. Since the dynamics of $z_3$ (which are decoupled from $z_1$ and $z_2$) render forward invariant (and UGAS) the set $\mathbb{T}^n$, the restriction only affects the states $(z_1,z_2)$. We divide the proof in two main steps. 

\vspace{0.1cm}
\noindent 
\textbf{Step 1: Average System.} For values of $\varepsilon_p$ sufficiently small, system \eqref{closed_loopESGeneral}, evolving in $C\times\mathbb{T}^n$, is in standard form for the application of averaging theory for dynamical systems with a continuous right-hand side. Using \cite[Lemma 7.1]{PovedaNaLi2019}, and standard arguments based on Taylor series expansions, we obtain the average system with state $z^A=[z_1^{A\top},z_2^{A\top}]^\top$ and dynamics
\begin{equation}\label{averagesystem}
\dot{z}^A_1= kF(z^A_1,z^A_2),~~\dot{z}^A_2=\frac{1}{\varepsilon_f}\left(-z^A_2+\nabla J(z^A_1)+\mathcal{O}(\varepsilon_a)\right),
\end{equation}
evolving in the set $C$. For small values of $\varepsilon_f>0$ system \eqref{averagesystem} is also in standard form for the application of averaging theory \cite{Wang:12_Automatica,PovedaNaLi2019}. To analyze this system, we set $\varepsilon_a=0$ in \eqref{averagesystem}, and we compute the reduced dynamics of the system, which in this case is precisely system \eqref{nominalAverage}. By \cite[Thm. 2]{Wang:12_Automatica} it follows directly that the set $\mathcal{A}\times\bar{M}\mathbb{B}$ is GPAS as $\varepsilon_f\to 0^+$ for system \eqref{averagesystem} with $\varepsilon_a=0$. By structural robustness results for ODEs with a continuous right-hand side \cite[Prop. A.1]{PovedaNaLi2019}, we obtain that system \eqref{averagesystem} renders the set $\mathcal{A}\times\bar{M}\mathbb{B}$ GPAS as $(\varepsilon_f,\varepsilon_a)\to 0^+$. We summarize with the following lemma.
\begin{lemma}\label{lemma1proof}
$\exists~\varepsilon_f^*>0$ s.t. $\forall~\varepsilon_f\in(0,\varepsilon_f^*)$ $\exists~\varepsilon_a^*>0$ s.t. $\forall~\varepsilon_a\in(0,\varepsilon_a^*)$, every solution of \eqref{averagesystem} satisfies
\begin{equation}\label{KLboundaverage1}
|z^A_1(t)|_{\mathcal{A}}\leq \beta_1(|z^A_1(0)|_{\mathcal{A}},t)+\frac{\nu}{4},~~  
\end{equation}
for all $t\in\text{dom}(z^A)$.  \hfill\qedsymbol
\end{lemma}
Let $\tilde{\mathcal{A}}:=\mathcal{A}\times\bar{M}\mathbb{B}$. Since system \eqref{averagesystem} is restricted to $C$, we have that $|z^A_2(t)|_{\bar{M}\mathbb{B}}=0$ for all $t\in\text{dom}(z^A)$, which implies that $|z^A(t)|_{\tilde{\mathcal{A}}}=|z^A_1(t)|_{\mathcal{A}}$ for all $t\in\text{dom}(z^A)$. Hence, it follows that
\begin{equation}\label{KLbound1}
|z^A(t)|_{\tilde{\mathcal{A}}}\leq \beta_1(|z^A(0)|_{\tilde{\mathcal{A}}},t)+\frac{\nu}{2},~t\in\text{dom}(z^A).  
\end{equation}
While this bound establishes a stability results for the (restricted) average system. It does not provide information about the existence of complete solutions. Nevertheless, the next lemma shows that system \eqref{averagesystem} generates solutions with unbounded time domains under appropriate initialization.
\begin{lemma}\label{complete_solutions}
$\exists~\varepsilon_f^*>0$ s.t. $\forall~\varepsilon_f\in(0,\varepsilon_f)~\exists~\varepsilon_a^*>0$ s.t. $\forall~\varepsilon_a\in(0,\varepsilon_a^*)$  every solution of system \eqref{averagesystem} (restricted to $C$) with $z^A(0)\in \left[(\mathcal{A}+\Delta\mathbb{B})\cap\mathcal{Z}\right]\times \Delta\mathbb{B}$, has an unbounded time domain.
\end{lemma}

\noindent 
\textbf{Proof}: Under the given condition on $z^A(0)$, by \eqref{KLboundaverage1} the trajectories $z^A_1$ of \eqref{averagesystem} satisfy $z^A_1(t)\in\text{int}(\mathcal{F}_s)$ for all $t\in\text{dom}(z^A)$. Moreover, this implies that $|z^A_1(t)|\leq M$ and $|\nabla J(z^A_1(t))+\mathcal{O}(\varepsilon_a)|<\tilde{M}$ for all $t\in\text{dom}(z^A)$, where without loss of generality we can take $|\mathcal{O}(\varepsilon_a)|<1$ for all $\varepsilon_a\in(0,\varepsilon_a^*)$. By Lemma \ref{auxiliarylemma}, this implies that $z_2^A(t)\in$ $\tilde{M}\mathbb{B}\subset\text{int}(\bar{M}\mathbb{B})$ for all $t\geq0$. Therefore, such trajectories satisfy $z^A(t)\in \text{int}(C)$ for all $t\geq0$, and have an unbounded time domain. \hfill$\blacksquare$    

\vspace{0.1cm}
Next, we establish a useful stability result for the average system \eqref{averagesystem}. The result makes use of the notion of Omega-limit sets of sets \cite[Def.6.23]{Goebel:12}.

\begin{lemma}\label{convergence}
$\exists~\varepsilon_f^*>0$ s.t. $\forall~\varepsilon_f\in(0,\varepsilon_f)~\exists~\varepsilon_a^*>0$ s.t. $\forall~\varepsilon_a\in(0,\varepsilon_a)$  there exists a compact set $\Omega(C)$ that is UGAS for system \eqref{averagesystem} restricted to $C$. \hfill\qedsymbol
% $\exists$ $T^*>0$ s.t. every solution $z^A$ of system \eqref{averagesystem} evolving in the compact $C$, with $z^A(0)\in \left[(\mathcal{A}+\Delta\mathbb{B})\cap\mathcal{Z}\right]\times \Delta\mathbb{B}$, satisfies
% %
% \begin{equation}
% |z^A_1(t)|_{\mathcal{A}}\leq \nu,~~ |z^A_2(t)|\leq \nu,
% \end{equation}
% %
% for all $t\geq T^*$.
\end{lemma}
\noindent 
\textbf{Proof:}  Let Lemma \ref{auxlemmagradient} generate $\delta$ using $\epsilon=\nu/8$, and let Lemmas \ref{lemma1proof} and \ref{complete_solutions} generate the pair $(\varepsilon_a,\varepsilon_f)$ such that \eqref{KLboundaverage1} holds with $\nu=\delta/4$, and such that $|\mathcal{O}(\varepsilon_a)|\leq \frac{\nu}{8}$. Choose $T'>0$ sufficiently large such that $\beta_1(\Delta,T')<\frac{\delta}{4}$. Such $T'$ always exists because $\beta\in\mathcal{K}\mathcal{L}$. By the exponential input-to-state stability of the low pass filter in \eqref{averagesystem} there exists $T''$ such that for all $t\geq T''$ the solutions of \eqref{averagesystem} with $z^A(0)\in \left[(\mathcal{A}+\Delta\mathbb{B})\cap\mathcal{Z}\right]\times \Delta\mathbb{B}$ satisfy
\begin{equation}
|z^A_2(t)|\leq \frac{\nu}{4}+\sup_{\tau\geq0} |\nabla J(z^A_1(\tau))+\mathcal{O}(\varepsilon_a)|.
\end{equation}
Thus, for all $t\geq T^*:=\max\{T',T''\}$ we have $$|z^A_2(t)|\leq \frac{\nu}{4}+\frac{\nu}{4}=\frac{\nu}{2},$$ and $|z^A_1(t)|\leq \frac{\nu}{2}$. Since such trajectories converge to a $0.5\nu$-neighborhood of $\mathcal{A}\times\{0\}$, the $\Omega$-limit set from $C$ is non-empty and satisfies $\Omega(C)\subset \left(\mathcal{A}\times\{0\}\right)+\frac{\nu}{2}\mathbb{B}\subset \text{int}(C)$. By \cite[Cor. 7.7]{Goebel:12} the set $\Omega(C)$ is UGAS for the average system \eqref{averagesystem} restricted to $C$. \hfill$\blacksquare$    

% \vspace{0.1cm}
% The next lemma establishes one additional useful property for system \eqref{averagesystem}.
% %
% \begin{lemma}\label{OmegaLimitSets}
% $\exists~\varepsilon_f^*>0$ s.t. $\forall~\varepsilon_f\in(0,\varepsilon_f)~\exists~\varepsilon_a^*>0$ s.t. $\forall~\varepsilon_a\in(0,\varepsilon_a)$ there exists a compact set $\Omega(C)$ that is UGAS for system \eqref{averagesystem} restricted to $C$.

% \end{lemma}
% %

% \noindent 
% \textbf{Proof}: By Lemmas \ref{complete_solutions} and \ref{convergence}, the $\Omega$-limit set from $C$ (\cite[Def. 6.23]{Goebel}) is non-empty and satisfies $\Omega(C)\subset \left(\mathcal{A}\times\{0\}\right)+\nu\mathbb{B}\subset \text{int}(C)$. Thus, by \cite[Cor. 7.7]{Goebel} the set $\Omega(C)$ is UGAS for \eqref{averagesystem} restricted to $C$. \hfill $\blacksquare$  

\vspace{0.1cm}

\noindent
\textbf{Step 2: Solutions of the Closed-Loop System.} We now study the behavior of system \eqref{closed_loopESGeneral} based on the properties of the average dynamics \eqref{averagesystem}. In particular, since the average system \eqref{averagesystem} (restricted to $C$) renders the set $\tilde{\mathcal{A}}$ SGPAS as $(\varepsilon_f,\varepsilon_a)\to 0^+$,  by averaging theory for perturbed systems \cite[Thm. 7]{PovedaNaLi2019} we directly obtain that for each pair of parameters $(\varepsilon_f,\varepsilon_a)$ inducing the bound \eqref{KLbound1}, there exists $\varepsilon_p^*>0$ such that for all $\varepsilon_p\in(0,\varepsilon_p^*)$ every solution $z$ of \eqref{closed_loopESGeneral} restricted to $C\times\mathbb{T}^n$ satisfies the bound
\begin{equation}\label{KL2bound}
|[z_1(t),z_2(t)]^\top|_{\tilde{\mathcal{A}}}\leq \beta_1(|[z_1(0),z_2(0)]^\top|_{\tilde{\mathcal{A}}},t)+\nu,   
\end{equation}
for all $\forall~t\in\text{dom}(z)$. Since for the restricted system we have that every solution $z$ satisfies
\begin{equation}\label{equalitybound}
\big|[z_1(t),z_2(t)]^\top\big|_{\tilde{\mathcal{A}}}=|z_1(t)|_{\mathcal{A}},~~\forall~t\in\text{dom}(z),
\end{equation}
we obtain the bound \eqref{KLboundTheorem}, which holds only for all $t\in\text{dom}(z)$.

\vspace{0.1cm}
\noindent 
Next, we leverage Lemmas \ref{complete_solutions} and \ref{convergence} to establish completeness of solutions for the original closed-loop system. To do this, we use the following lemma, corresponding to \cite[Thm. 1]{Wang:12_Automatica}.
\begin{lemma}\label{lemma_closeness_solutions}
Let $(\varepsilon_f,\varepsilon_a)>0$ such that Lemmas \ref{lemma1proof}-\ref{convergence} hold. Then, for each $\tilde{T},\epsilon>0$ there exists $\varepsilon_p^*$ such that for all $\varepsilon_p\in(0,\varepsilon_p^*)$ and all solutions $z$ of system \eqref{closed_loopESGeneral} (restricted to $C\times\mathbb{T}^n$) there exists a solution $z^A$ of system \eqref{averagesystem} (restricted to $C$),  such that for all $t\in\text{dom}(z)\cap\text{dom}(z^A)$:
\begin{equation}
\sup_{t\in[0,\tilde{T}]}|z_1(t)-z_1^A(t)|\leq \epsilon,~\sup_{t\in[0,\tilde{T}]}|z_2(t)-z_2^A(t)|\leq \epsilon.    
\end{equation}
\end{lemma}

The $\epsilon$-closeness property of Lemma \ref{lemma_closeness_solutions}, the stability result of Lemma \ref{convergence}, and the completeness property of the solutions of the average system, established in Lemma \ref{complete_solutions}, allow us to establish completeness of solutions for the original closed-loop system under the initial conditions of interest.
\begin{lemma}\label{last_lemma}
Let $(\varepsilon_f,\varepsilon_a)>0$ such that Lemmas \ref{lemma1proof}-\ref{convergence}. 
There exists $\varepsilon_p^*>0$ such that for all $\varepsilon_p\in(0,\varepsilon_p^*)$ there exists $T^{**}>0$ such that all solutions of system \eqref{closed_loopESGeneral} restricted to $C\times\mathbb{T}^n$, with $z(0)\in \left[(\mathcal{A}+\Delta\mathbb{B})\cap\mathcal{Z}\right]\times \Delta\mathbb{B}\times\mathbb{T}^n$ satisfy $z\in\text{int}(C)\times\mathbb{T}^n$ for all $t\geq0$, and
\begin{equation}
|z_1(t)|_{\mathcal{A}}\leq \nu,~~\text{and}~~|z_2(t)|\leq \nu,
\end{equation}
for all $t\geq T^{**}$.
\end{lemma}

\vspace{0.1cm}
\noindent
\textbf{Proof:} By Lemma \ref{convergence} there exists a function $\tilde{\beta}\in\mathcal{K}\mathcal{L}$ such that all solutions of \eqref{averagesystem} satisfy
\begin{equation}
|z^A(t)|_{\Omega(C)}\leq \tilde{\beta}(|z^A(0)|_{\Omega(C)},t),    
\end{equation}
for all $t\in\text{dom}(z)$. By \cite[Thm. 2]{Wang:12_Automatica}, there exists $\varepsilon_p^*$ such that for all $\varepsilon_p\in(0,\varepsilon_p^*)$ the solutions of \eqref{closed_loopESGeneral} (restricted to $C\times\mathbb{T}^n$) satisfy
\begin{equation}
|[z_1(t),z_2(t)]^\top|_{\Omega(C)}\leq \tilde{\beta}\left(|[z_1(0),z_2(0)]^\top|_{\Omega(C)},t\right)+\frac{\nu}{3},    
\end{equation}
for all $t\in\text{dom}(z)$. Thus, there exists $T^{***}>0$ such that $\big|[z_1(t),z_2(t)]^\top\big|_{\Omega(C)}\leq \frac{\nu}{2}$ for all $t\geq T^{**}$ such that $t\in\text{dom}(z)$. Since $\Omega(C)\subset \left(\mathcal{A}\times\{0\}\right)+\frac{\nu}{2}\mathbb{B}$, it follows that all solutions of \eqref{closed_loopESGeneral} satisfy 
\begin{equation}\label{final_bound_compact}
|z_1(t)|_{\mathcal{A}}\leq \nu,~~|z_2(t)|\leq \nu,
\end{equation}
for all $t\geq T^{***}$ such that $t\in\text{dom}(z)$. 

\vspace{0.1cm}
\noindent
Finally, we show that the set $\text{dom}(z)$ is unbounded for each solution of \eqref{closed_loopESGeneral} under the given initialization. Indeed, by Lemma \ref{complete_solutions}, under the given initialization all solutions of \eqref{averagesystem} remain in the interior of $C$. Moreover, by Lemma \ref{lemma_closeness_solutions}, all solutions of \eqref{closed_loopESGeneral} remain $\epsilon$-close to some solution of \eqref{averagesystem}, on compact time domains. Thus, there exists $\epsilon>0$ sufficiently small such that by applying Lemma \ref{lemma_closeness_solutions} with $\tilde{T}=T^{***}+1$ it follows that $(z_1(t),z_2(t))\in \text{int}(C)$ for all $t\in[0,T^{***}+1]$, and by \eqref{final_bound_compact} we have that $(z_1(t),z_2(t))\in \text{int}(C)$ for all $t\geq T^{***}$. The combination of these bounds establishes the result.  \null\hfill\null $\blacksquare$

The result of Theorem \ref{general_theoremES} follows by the bound \eqref{KL2bound}, the relation \eqref{equalitybound},  and the result of Lemma \ref{last_lemma}.
